# Supplementary material for: zkVC: Fast Zero-Knowledge Proof for Private and Verifiable Computing
Source: arXiv:2504.12217 source file (2025-04-16)
Supplement: Supplementary file 1 [file appendix.tex]

\section{Proof for CRPC}
We provide a detailed definition of CRPC and present proof establishing the equivalence between CRPC and the original matrix multiplication. We denote by $[[n]]$ the set $\{0,...,n-1\}$. We use lower-case letters with a “hat” and a "tilde" symbol such as $\hat{a}$ and $\tilde{a}$ to represent polynomials, and $\hat{a}[j]$ to denote $j$-th coefficient of $\hat{a}$. We denote the $k$-th column of matrix $M$ as $M[:,k]$, and $k$-th row as $M[k,:]$.

For general matrix multiplication \(Y^{a \times b} = X^{a \times n} \times W^{n \times b}\), we define three mapping functions $\pi_1^x, \pi_1^w: \mathbb{R} \rightarrow \mathbb{F}_{d,p}$, that maps a vector to a polynomial of degree $d$ over finite field defined by prime $p$, and $\pi_2: \mathbb{R}^2 \rightarrow \mathbb{F}_{d,p}$, that maps a matrix accordingly. Specifically, we have
\begin{equation*}
\begin{aligned}
&\hat{x}_k = \pi_1^{x}(X[:,k]), where\ \hat{x}_k[i\cdot b] = X[i,k] \\
&\hat{w}_k = \pi_1^{w}(W[k,:]), where\ \hat{w}_k[j] = W[k,j] \\
&\hat{y} = \pi_2^{y}(Y), where\ \hat{y}[i\cdot b + j] = Y[i,j]
\end{aligned}
\end{equation*}
where  $i\in [[a]]\ $, $ j\in [[b]], k\in [[n]]$ and all other coefficients of  $\hat{x}_k, \hat{w}_k, \hat{y}$ are set to $0$. Note that $\hat{x}_k, \hat{w}_k, \hat{y}$ are all polynomials of a random variable $Z \in \mathbb{F}_p^*$. In our setting, the degree $d$ of a polynomial is $a\cdot b$.

\noindent \textbf{Proposition 1.} Given two matrices $X, W$ and it's mappings $\{\hat{x}_k = \pi_1^{x}(X[:,k])\}_{k=0}^{n-1}$,  $\{\hat{w}_k =\pi_1^{w}(W[k,:]) \}_{k=0}^{n-1} \in \mathbb{F}_{d,p}$, the matrix multiplication $Y = X \times W$ is satisfied if and only if the polynomial multiplication $\hat{y} = \sum_{k=0}^{n-1} (\hat{x}_k\hat{w}_k) $ is satisfied. That is, $Y[i,j]$ is computed in $\hat{y}[i\cdot b + j]$ for all $i\in [[a]]\,\ j\in [[b]]$.

\begin{proof}
\label{proof:poly}
($\Rightarrow$) If $Y = X \times W$ is satisfied, we have $Y[i,j]=\sum_{k=0}^{n-1}(X[i,k]\cdot W[k,j])$. Because $\hat{y}[i\cdot b + j] = Y[i,j]$, we have $\hat{y}[i\cdot b + j] = \sum_{k=0}^{n-1}(X[i,k]\cdot W[k,j]) = \sum_{k=0}^{n-1}(\hat{x}_k[i]\cdot \hat{w}_k[j])$. Accordingly, for all $i\in [[a]]\ and j\in [[b]]$, we then have $\hat{y} = \sum_{k=0}^{n-1} (\hat{x}_k\hat{w}_k) $, which means the polynomial multiplication is satisfied.

($\Leftarrow$) 
For simplicity, we employ a proof by contradiction. Assume the polynomial multiplication $\hat{y} = \sum_{k=0}^{n-1} (\hat{x}_k\hat{w}_k)$ is satisfied, but the matrix multiplication $Y = X \times W$ is not. This means that $\hat{y}$ corresponds to some matrix $\Bar{Y}$ with $\Bar{Y} \neq X \times W$. Let $\tilde{y} = \pi_2^{y}(Y)$ be the polynomial corresponding to the correct matrix multiplication. We have $\tilde{y}[i\cdot b + j] = Y[i,j] = \sum_{k=0}^{n-1}(X[i,k]\cdot W[k,j]) = \sum_{k=0}^{n-1}(\hat{x}_k[i]\cdot \hat{w}_k[j])$. Thus, $\tilde{y} = \sum_{k=0}^{n-1} (\hat{x}_k\hat{w}_k) = \hat{y}$ accordingly. This means $\tilde{y}$ must coincide with $\hat{y}$ at some random point $Z$. However, because $\Bar{Y} \neq Y$, at least one element $\Bar{Y}[i,j]$ differs, implying $\tilde{y}$ and $\hat{y}$ represent different polynomials. 

Consider the nonzero polynomial $p = \tilde{y} - \hat{y}$. By the Schwartz-Zippel Lemma, the probability that $p$ evaluates to zero at a uniformly random point $Z$ from a sufficiently large field is negligible. 

Hence, if $\tilde{y}$ and $\hat{y}$ yield the same value at a random point $Z$, it's almost certain they're not different polynomials. This implies $\Bar{Y} = Y$, which is a contradiction. Thus, if polynomial multiplication $\hat{y} = \sum_{k=0}^{n-1} (\hat{x}_k\hat{w}_k)$ is satisfied, matrix multiplication $Y = X \times W$ is also satisfied.
\end{proof}

% In our setting specifically, the highest degree $d$ is $a\cdot b$, while $\left | S \right |$ is the size of the finite field (eg. $2^{127}$).

\noindent \textbf{Lemma 1.} The Schwartz-Zipplel Lemma. Let $p(x_1,...,x_n)$ be a non-zero polynomial of $n$ variables with degree $d$. Let $S$ be a finite subset of $\mathbb{R}$, with at least d elements in it. If we assign $x_1,...,x_n$ values from $S$ independently and uniformly at random, then
\begin{equation*}
\begin{aligned}
\mathbb{P}[ p(x_1,...,x_n)=0 ] \leq \frac{d}{\left | S \right | }
\end{aligned}
\end{equation*}

\section{R1CS}
\noindent \textbf{Definition 1. Rank-1 Constraint System (R1CS).} An R1CS instance consists of size bounds $n,m,N,l \in \mathbb{N}$ where $m>l$, three matrices $A,B,C \in \mathbb{F}^{n\times m}$ with at most $N = \Omega(max(n, m))$ non-zero entries in total and a public vector $x\in \mathbb{F}^l.$ An R1CS witness consists of a private vector $w\in \mathbb{F}^{m-l-1}.$ An R1CS instance $(A,B,C,x)$ is satisfied by an R1CS witness $w$ if:
\begin{equation}
(A\cdot z) \circ (B\cdot z) = (C\cdot z)
\end{equation}
where $z=(1,v,w) \in \mathbb{F}^m$, $\circ$ is the Hadamard (i.e, entry-wise product) product, $\cdot$ is the matrix-vector product.
